# Supplementary material for: Merging multiple input descriptors and supervisors in a deep neural network for tractogram filtering
Source: arXiv:2307.05786 source file (2023-07-11)
Supplement: Supplementary file 1 [file appendix.tex]

%
% let's just take out this for the thesis' version.
\begin{comment}

\appendix
%
\section{Dataset}
%
\label{app:dataset}
%
\begin{table}[]
    \centering
    \caption{Composition of our data sets. Subjects are identified by their subject id in the Human Connectome Project (HCP).}    \begin{tabular}{cccccc}
        \toprule
        id & split 1 & split 2 & split 3 & split 4 & split 5 \\
        \midrule
        599671 & train & & & & \\
        622236 & valid & & & & \\
        665254 & train & & & & \\
        672756 & train & & & & \\
        690152 & & & & & \\
        702133 & & & & & \\
        734045 & & & & & \\
        751348 & & & & & \\
        779370 & & & & & \\
        784565 & & & & & \\
        833249 & & & & & \\
        837964 & & & & & \\
        871762 & & & & & \\
        871964 & & & & & \\
        899885 & & & & & \\
        901442 & & & & & \\
        904044 & & & & & \\
        922854 & & & & & \\
        978578 & & & & & \\
        987983 & & & & & \\
        \bottomrule
    \end{tabular}

    \label{tab:dataset}
\end{table}
\end{comment}
